# Supplementary material for: Prospects for a lattice calculation of the rare decay $\Sigma^+\to p\ell^+\ell^-$
Source: arXiv:2209.15460 source file (2023-05-03)
Supplement: Supplementary file 1 [file appendix.tex]

%%%%%%%%%%%%%%%%%%%%%%%%%%%%%%%%%%%%%%%%%%%%%%%%%%
%
%Appendix
%
%%%%%%%%%%%%%%%%%%%%%%%%%%%%%%%%%%%%%%%%%%%%%%%%%%
%
%
%
%\newpage
\section{Traces of the integrated correlator}
\label{sec:traces}
In the following we give examples of traces $\mathrm{Tr}[\Gamma F_\mu(\vec{p},\vec{k})]$ and combinations that can be used to extract the form factors $a(q^2)$, $b(q^2)$, $c(q^2)$ and $d(q^2)$. Recall from section \ref{sec:amplitude} that
\begin{equation}
 F_\mu(\vec{p},\vec{k}) \equiv -i\,\lim\limits_{T_{a,b}\rightarrow\infty}\overline{I}_\mu(T_a,T_b;\vec{p},\vec{k}) = \left(\slashed{p} + iM_N\right)\, \tilde{\mathcal{A}}_\mu(q^2)\, \left(\slashed{k} + iM_{\Sigma^+}\right)
\end{equation}
with 
\begin{equation}
 \tilde{\mathcal{A}}_\mu(q^2) = i\sigma_{\nu\mu}q^\nu \left(a(q^2)+\gamma_5 b(q^2)\right) + 
\left(q^2\gamma_\mu-q_\mu \slashed{q}\right)\left(c(q^2)+\gamma_5 d(q^2)\right)\,.
\end{equation}
The traces for some of the $\Gamma$-matrices are given by
\begin{equation}
 \begin{aligned}
  \mathrm{Tr}\left[\mathds{1} F_\mu\right] = &\Big[2(q\cdot p)k_\mu - 2(q\cdot k)p_\mu \Big]a(q^2)\\
  &+ 4\Big[iM_{\Sigma^+}(q^2p_\mu-(p\cdot q)q_\mu)+iM_N(q^2k_\mu-(k\cdot q)q_\mu) \Big]c(q^2)
 \end{aligned}
\end{equation}
 \begin{equation}
   \begin{aligned}
  \mathrm{Tr}\left[\gamma_5 F_\mu\right] = &\Big[2(q\cdot k)p_\mu - 2(q\cdot p)k_\mu \Big]b(q^2)\\
  &+ 4\Big[iM_{\Sigma^+}(q^2p_\mu-(p\cdot q)q_\mu)-iM_N(q^2k_\mu-(k\cdot q)q_\mu) \Big]d(q^2)
 \end{aligned}
\end{equation}
  \begin{equation}
   \begin{aligned}
  \mathrm{Tr}\left[\gamma_\rho F_\mu\right] = &\Big[2iM_{\Sigma^+}(\delta_{\rho\mu}(q\cdot p)-q_\rho p_\mu) - 2i M_N(\delta_{\rho\mu}(q\cdot k)-q_\rho k_\mu) \Big]a(q^2)\\
  &+ \Big[2ik_\tau p_\nu M_N \epsilon^{\tau\rho\nu\mu} -2ik_\nu p_\sigma M_{\Sigma^+} \epsilon^{\rho\sigma\nu\mu} \Big]b(q^2)\\
  &+ \Big[4(p_\rho k_\mu q^2 - \delta_{\rho\mu}(p\cdot k)q^2+q^2k_\rho p_\mu - p_\rho(k\cdot q)q_\mu + (p\cdot k) q_\mu q_\rho - (p\cdot q)k_\rho q_\mu)\\
  &\qquad-4M_{\Sigma^+} M_N q^2\delta_{\rho\mu}+4M_{\Sigma^+} M_N q_\mu q_\rho \Big]c(q^2)\\
  &+ \Big[-4q^2p_\sigma k_\tau \epsilon^{\tau\rho\sigma\mu}\Big]d(q^2)
 \end{aligned}
\end{equation}
   \begin{equation}
   \begin{aligned}
  \mathrm{Tr}\left[\gamma_5\gamma_\rho F_\mu\right] = &\Big[-2ik_\nu p_\sigma M_{\Sigma^+} \epsilon^{\rho\sigma\nu\mu} + 2iM_Np_\nu k_\tau \epsilon^{\rho\nu\mu\tau}\Big]a(q^2)\\
  &+ \Big[ 2iM_{\Sigma^+}(\delta_{\mu\rho}(p\cdot q)-p_\mu q_\rho)+2iM_N(\delta_{\mu\rho}(k\cdot q)-k_\mu q_\rho)\Big]b(q^2)\\
  &+ \Big[-4p_\sigma k_\tau q^2 \epsilon^{\rho\sigma\mu\tau} \Big]c(q^2)\\
  &+ \Big[-4q^2 \big(p_\rho k_\mu-\delta_{\rho\mu}(p\cdot k)+p_\mu k_\rho\big) +4q_\mu \big(p_\rho(k\cdot q)-q_\rho (p\cdot k) + k_\rho(p\cdot q)\big) \\
  &\qquad + 4M_N M_{\Sigma^+} \big(q_\mu q_\rho-q^2\delta_{\mu\rho}\big)\Big]d(q^2)\,.
 \end{aligned}
\end{equation}
The traces can be written in the general form
 \begin{equation}
 \mathrm{Tr}\left[\Gamma F_\mu\right] \equiv a^\Gamma_\mu a(q^2) + b^\Gamma_\mu b(q^2) + c^\Gamma_\mu c(q^2) +d^\Gamma_\mu d(q^2) 
 \label{eq:abcdcoef}
\end{equation}
with coefficients $a_\Gamma$, $b_\Gamma$, $c_\Gamma$ and $d_\Gamma$. In the following we will give an explicit example of combinations of traces that can be used to extract the four form factors for a specific kinematics\footnote{This is to give an explicit example and other kinematics are possible as well.}, where the $\Sigma$ is at rest $\vec{k}=0$ and the nucleon is moving with $\vec{p}=(p_x,0,0)$.
\subsection{Example: $\Sigma$ at rest}
For the $\Sigma$ at rest and moving nucleon the (Euclidean) four momenta are given by $k=(iM_{\Sigma^+}, \vv{0})$ and $p=(iE_N,\vec{p})$ with $E_N=\sqrt{M_N^2+\vec{p}^2}$. Some of the coefficients as defined in eq.~\eqref{eq:abcdcoef} are given by\footnote{In the following there is no sum over repeated indices $j$ or $\mu$.}
\begin{itemize}
 \item $\mathrm{Tr}\left[F_\mu\right]$:
\begin{align}
 &a^{\mathds{1}}_0 = -2iM_{\Sigma^+}\, \vv{p}^2 \hspace{2.0cm}
 &&a^{\mathds{1}}_j = 2\,M_{\Sigma^+}(M_{\Sigma^+}- E_N)\,p_j\\
 &c^{\mathds{1}}_0 = -4M_{\Sigma^+}(M_N+M_{\Sigma^+})\,\vv{p}^2 &\hspace{1.5cm} &c^{\mathds{1}}_j = 4i\,M_{\Sigma^+}(E_N-M_{\Sigma^+})(M_N+M_{\Sigma^+})\,p_j\\
 &b^{\mathds{1}}_\mu = 0  \hspace{2.0cm}&&d^{\mathds{1}}_\mu = 0
\end{align}
 \item $\mathrm{Tr}\left[\gamma_5 F_\mu\right]$:
\begin{align}
 &b^{\gamma_5}_0 = 2i\, M_{\Sigma^+} \vv{p}^2\hspace{2.0cm}
 &&b^{\gamma_5}_j = 2 M_{\Sigma^+}(E_N-M_{\Sigma^+}) p_j\\
 &d^{\gamma_5}_0 = 4 M_{\Sigma^+} (M_N-M_{\Sigma^+}) \vv{p}^2&\hspace{1.5cm}
 &d^{\gamma_5}_j = 4 i M_{\Sigma^+}(E_N-M_{\Sigma^+})(M_{\Sigma^+}-M_N) p_j\\
 &a^{\gamma_5}_\mu = 0 \hspace{2cm}&&c^{\gamma_5}_\mu = 0
 \end{align}
 \item $\mathrm{Tr}\left[\gamma_\mu F_\mu\right]$:
 \begin{align}
 &a^{\gamma_0}_0 = -2 i M_{\Sigma^+} \vv{p}^2\\
 &a^{\gamma_j}_j = -2 i M_{\Sigma^+} \left[(\vv{p}^2-p_j^2) + (E_N-M_N)(M_{\Sigma^+}-E_N)\right]\\
 &c^{\gamma_0}_0 = -4 M_{\Sigma^+} (M_N+M_{\Sigma^+}) \vv{p}^2\\
 &c^{\gamma_j}_j = -4M_{\Sigma^+} \left\{ (E_N-M_N)  \left[(E_N-M_{\Sigma^+})^2-(\vv{p}^2-p_j^2)\right] - (E_N-M_{\Sigma^+}) p_j^2\right\}\\
 &b^{\gamma_\mu}_\mu = 0\hspace{4cm}d^{\gamma_\mu}_\mu = 0
\end{align}
 \item $\mathrm{Tr}\left[\gamma_5\gamma_\mu F_\mu\right]$:
 \begin{align}
 &b^{\gamma_5\gamma_0}_0 = -2 i M_{\Sigma^+} \vv{p}^2\\
 &b^{\gamma_5\gamma_j}_j = -2 i M_{\Sigma^+} \left[(\vv{p}^2-p_j^2) + (E_N+M_N) (M_{\Sigma^+}-E_N) \right]\\
 &d^{\gamma_5\gamma_0}_0 = -4 M_{\Sigma^+} (M_N-M_{\Sigma^+}) \vv{p}^2\\
 &d^{\gamma_5\gamma_j}_j = 4 M_{\Sigma^+} \left\{(E_N+M_N) \left[(E_N-M_{\Sigma^+})^2-(\vv{p}^2-p_j^2)\right]-(E_N-M_{\Sigma^+}) p_j^2\right\}\\
 &a^{\gamma_5\gamma_\mu}_\mu = 0 \hspace{4cm}c^{\gamma_5\gamma_\mu}_\mu = 0
 \end{align}
\end{itemize}
As a specific example, we will now turn to the case $\vec{p}=(p_x,0,0)$, i.e.\ the momentum of the nucleon is in $x-$direction. It is straightforward to show that the four form factors can be extracted from\footnote{This is just an example, and other combinations of traces are possible as well.} 
  \begin{equation}
  a(q^2) = \frac{c^{\gamma_2}_2 \mathrm{Tr}\left[F_0\right]-c^{\mathds{1}}_0\mathrm{Tr}\left[\gamma_2 F_2\right]}{a^\mathds{1}_0 c^{\gamma_2}_2-c^\mathds{1}_0 a^{\gamma_2}_2}
  \label{eq:getak0j}
  \end{equation}
    \begin{equation}
   b(q^2) = \frac{d^{\gamma_5\gamma_2}_2 \mathrm{Tr}\left[\gamma_5 F_0\right]-d^{\gamma_5}_0\mathrm{Tr}\left[\gamma_5\gamma_2 F_2\right]}{b^{\gamma_5}_0 d^{\gamma_5\gamma_2}_2-d^{\gamma_5}_0 b^{\gamma_5\gamma_2}_2}
   \label{eq:getbk0j}
  \end{equation}
      \begin{equation}
   c(q^2) = \frac{a^{\gamma_2}_2 \mathrm{Tr}\left[F_0\right]-a^{\mathds{1}}_0\mathrm{Tr}\left[\gamma_2 F_2\right]}{c^\mathds{1}_0 a^{\gamma_2}_2-a^\mathds{1}_0 c^{\gamma_2}_2}
    \label{eq:getc0j} 
  \end{equation}
    \begin{equation}
   d(q^2) = \frac{b^{\gamma_5\gamma_2}_2 \mathrm{Tr}\left[\gamma_5 F_0\right]-b^{\gamma_5}_0\mathrm{Tr}\left[\gamma_5\gamma_2 F_2\right]}{d^{\gamma_5}_0 b^{\gamma_5\gamma_2}_2-b^{\gamma_0}_2 d^{\gamma_5\gamma_2}_2}
   \label{eq:getd0j}
  \end{equation}
  with the denominators of equations \eqref{eq:getak0j}-\eqref{eq:getd0j}
  \begin{align}
   &a^\mathds{1}_0 c^{\gamma_2}_2-c^\mathds{1}_0 a^{\gamma_2}_2= b^{\gamma_5}_0 d^{\gamma_5\gamma_2}_2-d^{\gamma_5}_0 b^{\gamma_5\gamma_2}_2 = -16i\,M_{\Sigma^+}^2\,p_x^4\\
  & b^{\gamma_5}_0 d^{\gamma_5\gamma_2}_2-d^{\gamma_5}_0 b^{\gamma_5\gamma_2}_2 = d^{\gamma_5}_0 b^{\gamma_5\gamma_2}_2-b^{\gamma_0}_2 d^{\gamma_5\gamma_2}_2 = 16i\,M_{\Sigma^+}^2\,p_x^4\,.
  \end{align}

\newpage
\section{Feynman Diagrams for the rare Hyperon Decay}
\label{sec:appWick}
In the following, we show the diagrams corresponding to the different Wick contractions of the four-point function $ \Gamma^{(4)}_\mu$ defined in eq.~\eqref{eq:fourptHJ}. There are six different contractions for each of the four topologies of the three-point function \eqref{eq:threeptH}.
\begin{figure}[h]
\centering
 \includegraphics[width=0.9\textwidth]{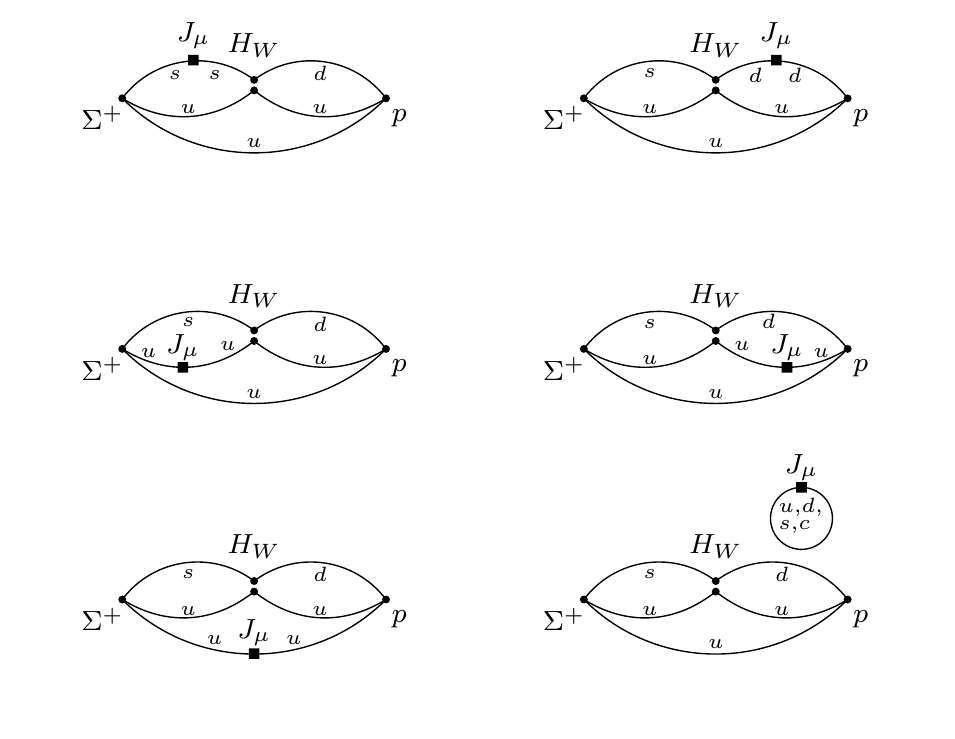}
 \caption{Four-point diagrams for the $C_{sd}$ class. The squared vertex shows the insertion of the electromagnetic current $J_\mu$.}
 \label{fig:Csd4pt}
\end{figure}
\newpage
\begin{figure}[h]
\centering
 \includegraphics[width=0.9\textwidth]{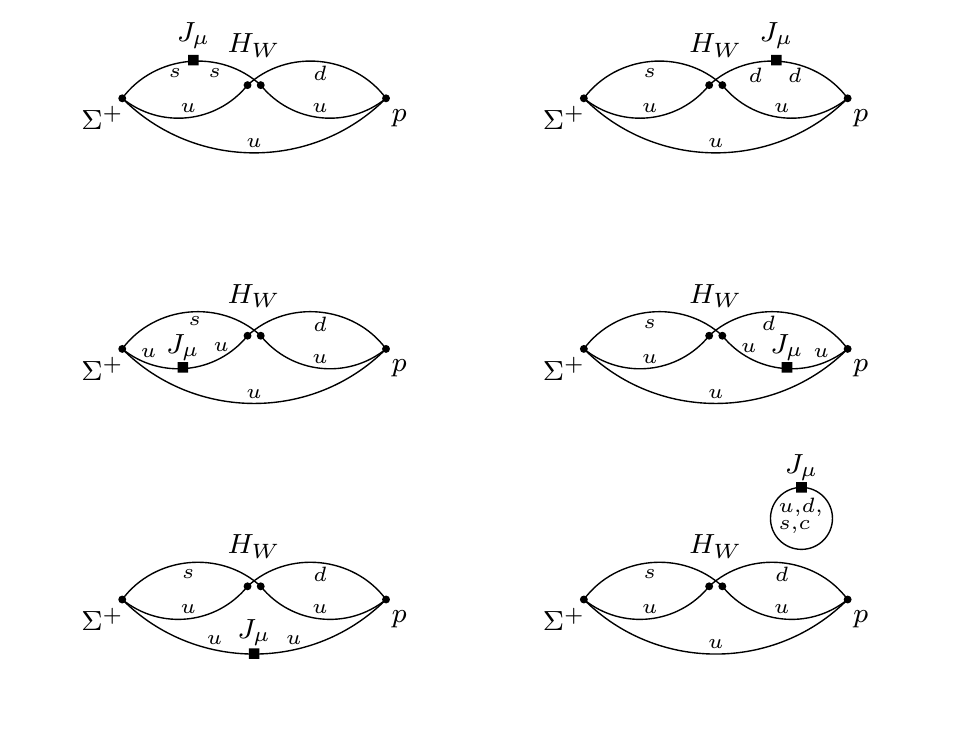}
 \caption{Four-point diagrams for the $C_{su}$ class. The squared vertex shows the insertion of the electromagnetic current $J_\mu$.}
  \label{fig:Csu4pt}
\end{figure}
\newpage
\begin{figure}[h]
\centering
 \includegraphics[width=0.9\textwidth]{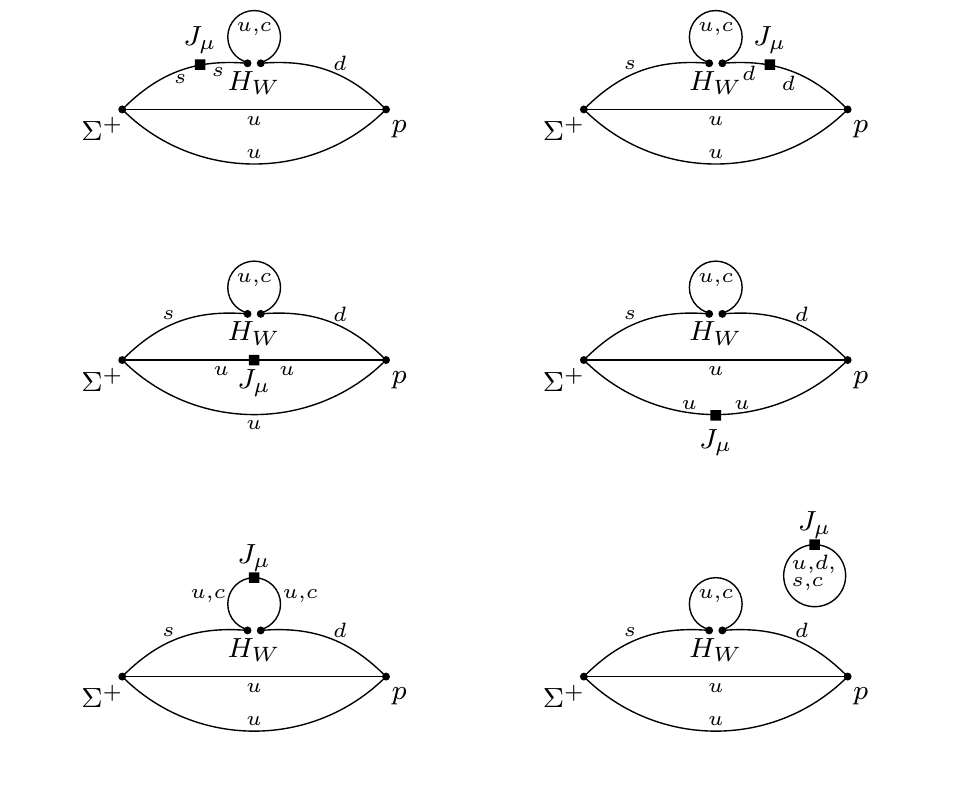}
 \caption{Four-point diagrams for the $S$ class. The squared vertex shows the insertion of the electromagnetic current $J_\mu$.}
  \label{fig:S4pt}
\end{figure}
\newpage
\begin{figure}[h]
\centering
 \includegraphics[width=0.9\textwidth]{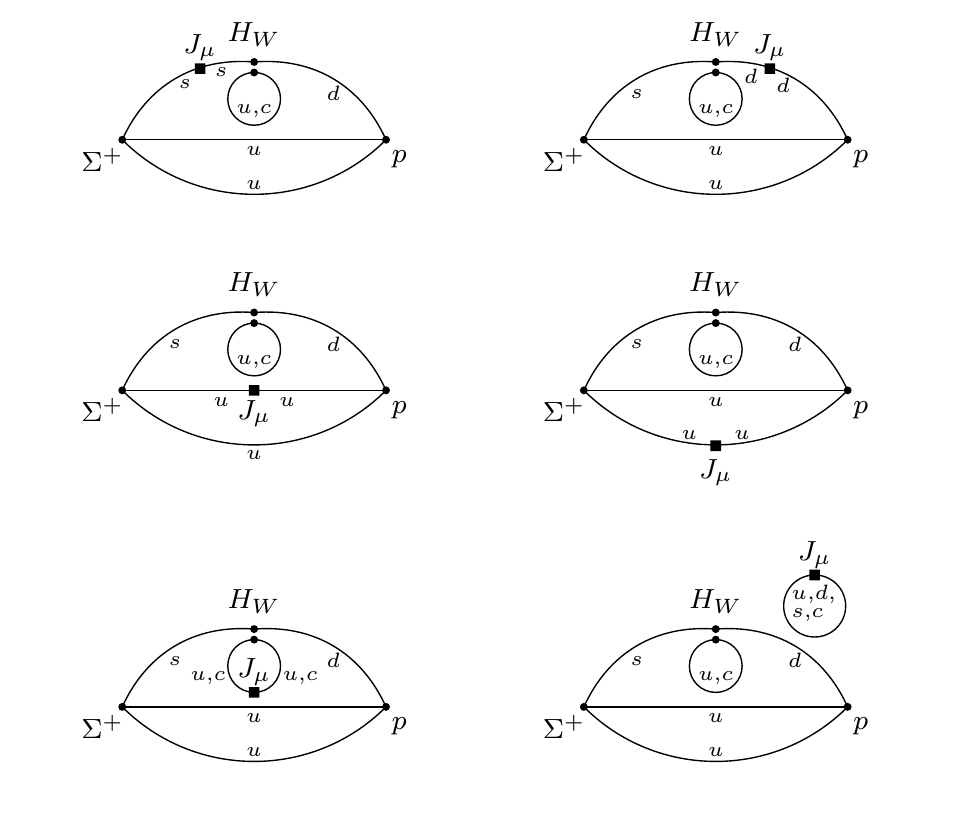}
 \caption{Four-point diagrams for the $E$ class. The squared vertex shows the insertion of the electromagnetic current $J_\mu$.}
  \label{fig:E4pt}
\end{figure}
